# Supplementary material for: Polyatomic candidates for cooling of molecules with lasers from simple theoretical concepts
Source: arXiv:1504.08326 ancillary file (2016-03-21)
Supplement: Supplementary file 1 [file Supplementary-arxiv-9i.pdf]

# Supplementary material for MS "Polyatomic candidates for cooling of molecules with lasers from simple theoretical concepts"

Timur Isaev* and Robert Berger
*Fachbereich Chemie, Philipps-Universität Marburg, 35032, Marburg, Hans-Meerwein-Str 4, Germany*
(Dated: March 6, 2016)

* NRC KI Petersburg Nuclear Physics Institute, 188300, Gatchina, Orlova Roscha 1, Russia

TABLE I. Calculated and experimental molecular parameters and FC factors for CaOH and CaNC. For CaOH the results of the calculations which best reproduce the experimental internuclear distance $R_{(\mathrm{Ca-O})}$ are presented (MCSCF/def2-QZVPP). For CaNC the results of MCSCF calculations with the def2-QZVPP basis set are given. See manuscript text for discussion on stability/accuracy of FC factors and tables below for additional data. Internuclear distances $R_i$ are given in Å, electric dipole moments in Debye, transition wavenumbers $T_\mathrm{e}$ and harmonic vibrational wavenumbers $\tilde{\omega}_\mathrm{e}$ of normal mode $\nu_l$ in inverse centimeters. For FC factors the corresponding vibrational quantum numbers are reported, e.g $1_2^0$ is FC factor for a vibronic transition between the ground (0) vibrational state of the excited electronic state and the vibrational state with the first mode (1) (Ca-X stretching) being doubly excited (2) in the ground electronic state. The irreducible representation $\pi$ is two-dimensional, but the degeneracy is slightly lifted in the numerical calculations. Thus, we provide vibrational wavenumbers of both components.

| | CaOH | | | | CaNC | | |
|---|---|---|---|---|---|---|---|
| State | Calculation | | Experiment[a] | State | Calculation | | Experiment[b] |
| X ($^2\Sigma$) | $R_{(\mathrm{Ca-O})}$ | 2.0038 | 1.9746 | X ($^2\Sigma$) | $R_{(\mathrm{Ca-N})}$ | 2.2344 | 2.2065 |
| | $R_{(\mathrm{O-H})}$ | 0.9333 | 0.9562 | | $R_{(\mathrm{N-C})}$ | 1.1866 | 1.1186 |
| | ∠ Ca-O-H | 179.97 | 180.00 | | ∠ Ca-N-C | 179.54 | 180.00 |
| | $\lvert D\rvert$ | 0.42[c] | 1.465[d] | | $\lvert D\rvert$ | 6.08 | 6.84 |
| A ($^2\Pi$) | $R_{(\mathrm{Ca-O})}$ | 1.9769 | 1.9532 | A ($^2\Pi$) | $R_{(\mathrm{Ca-N})}$ | 2.2076 | – |
| | $R_{(\mathrm{O-H})}$ | 0.9332 | 0.9572 | | $R_{(\mathrm{N-C})}$ | 1.1861 | – |
| | ∠ Ca-O-H | 179.97 | 180.00 | | ∠ Ca-N-C | 179.97 | – |
| | $\lvert D\rvert$ | 0.25 | 0.836[d] | | $\lvert D\rvert$ | 5.91 | 6.10 |
| | $T_\mathrm{e}$ | $15\times10^3$ | $T_{00}$ 15998[e] | | $T_\mathrm{e}$ | $16\times10^3$ | $T_{00}$ 16299 |
| FC factors | 0.9213[f], 0.0763[g], 0.0019[h] | | | FC factors | 0.9092[i], 0.0664[j], 0.02025[k] | | |
| $\sum$ | $> 0.999$ | | | $\sum$ | 0.9959 | | |
| | Normal modes $\nu_l$ | | | | Normal modes $\nu_l$ | | |
| X ($^2\Sigma$) | $\nu_3(\sigma^+)$ | 4276 | | X ($^2\Sigma$) | $\nu_3(\sigma^+)$ | 2062 | |
| | $\nu_1(\sigma^+)$ | 622 | | | $\nu_1(\sigma^+)$ | 412 | |
| | $\nu_2(\pi)$ | 411/408 | | | $\nu_2(\pi)$ | 85/85 | |
| A ($^2\Pi$) | $\nu_3(\sigma^+)$ | 4279 | | A ($^2\Pi$) | $\nu_3(\sigma^+)$ | 2066 | |
| | $\nu_1(\sigma^+)$ | 646 | | | $\nu_1(\sigma^+)$ | 426 | |
| | $\nu_2(\pi)$ | 402/386 | | | $\nu_2(\pi)$ | 63/63 | |

[a] from [1]
[b] from [2], only data for X state are available
[c] in previous investigation in [3] the calculated electric dipole moment for X state is also considerably smaller than experimentally measured, the reason for such a big discrepancy probably connected with the compensation of the large dipole moment form the ionic core by charge distribution from the valence electron
[d] from [4]
[e] from [5]
[f] $0_0^0$
[g] $1_1^0$ Ca−OH stretching
[h] $1_2^0$ Ca−OH stretching
[i] $0_0^0$
[j] $1_1^0$ Ca−NC stretching
[k] $2_2^0$ bending mode

TABLE II. Calculated and experimental molecular parameters and FC factors for $MgCH_3$ and $CaCH_3$. Internuclear distances $R_i$ are given in Å, electric dipole moments in Debye, transition wavenumbers $T_e$ and harmonic vibrational wavenumbers $\tilde{\omega}_e$ of normal mode $\nu_l$ in inverse centimetres. Only wavenumbers for totally-symmetric modes are provided. FC factors are designated analogously to Table I.

| $MgCH_3$ | | | | $CaCH_3$ | | | |
|---|---|---|---|---|---|---|---|
| State | | Calculation[a] | Experiment[b] | State | | Calculation[c] | Experiment[d] |
| X ($^2A_1$) | $R_{(Mg-C)}$ | 2.1204(2.1205) | 2.102 | X ($^2A_1$) | $R_{(Ca-C)}$ | 2.4206 | 2.349 |
| | $R_{(C-H1)}$ | 1.0932(1.0931) | 1.105[e] | | $R_{(C-H)}$ | 1.1095 | 1.100 |
| | $R_{(C-H2)}$ | 1.0932(1.0931) | 1.105 | | $\lvert D\rvert$ | 2.21 | 2.62[f] |
| | $R_{(C-H3)}$ | 1.0932(1.0931) | 1.105 | | | | |
| | $\lvert D\rvert$ | 0.91 (0.91) | 0.76 [g] | | | | |
| A ($^2E$) | $R_{(Mg-C)}$ | 2.1636(2.1629) | 2.124 | A ($^2E$) | $R_{(Ca-C)}$ | 2.4052 | 2.353 |
| | $R_{(C-H1)}$ | 1.085(1.084) | 1.105 | | $R_{(C-H)}$ | 1.0892 | 1.100 |
| | $R_{(C-H2)}$ | 1.085(1.084) | 1.105 | | | | – |
| | $R_{(C-H3)}$ | 1.085(1.087) | 1.105 | | | | |
| | $\lvert D\rvert$ | 0.92 (0.93) | – | | $\lvert D\rvert$ | 2.16 | 1.69[f] |
| | $T_e$ | $21\times10^3$ | $T_{00}$ 20030 | | $T_e$ | $14\times10^3$ | $T_{00}$ 14743 |
| FC factors | 0.7090 (0.6714)[h], 0.19218(0.1728)[i], 0.02635 (0.03271)[m] | | | FC factors | 0.9079[j], 0.0509[k], 0.03718[l] | | |
| $\sum$ | 0.9275 (0.8769) | | | | $\sum$ | 0.9960 | |
| | | Normal modes $\nu_l$ | | | | Normal modes $\nu_l$ | |
| X ($^2A_1$) | $\nu_1(a_1)$ | 3043 | | X ($^2A_1$) | $\nu_1(a_1)$ | 3035 | |
| | $\nu_2(a_1)$ | 1154 | | | $\nu_2(a_1)$ | 1187 | |
| | $\nu_3(a_1)$ | 511 | | | $\nu_3(a_1)$ | 418 | |
| A ($^2E$) | $\nu_1(a_1)$ | 2605 | | A ($^2E$) | $\nu_1(a_1)$ | 2863 | |
| | $\nu_2(a_1)$ | 1089 | | | $\nu_2(a_1)$ | 1153 | |
| | $\nu_3(a_1)$ | 443 | | | $\nu_3(a_1)$ | 435 | |

[a] MCSCF/CI calculation in $C_{3v}$ symmetry, results without accounting for symmetry (including non-symmetrical modes in FC factors) are in parenthesis
[b] from [6]
[c] MCSCF calculations in $C_{3v}$ symmetry
[d] from [7]
[e] in [6] this value is fixed from theoretical calculations by G.Gawboy
[f] from [8]
[g] prediction from [8]
[h] $0_0^0$
[i] $2_1^0(5_1^0)$ umbrella mode
[j] $0_0^0$
[k] $2_1^0$ Ca−$CH_3$ stretching mode
[l] $3_1^0$ umbrella mode
[m] $2_1^0 3_1^0$ $(5_2^0)$ stretching Mg−$CH_3$ + umbrella modes

TABLE III. Electric transition dipole moments (TDM) in Debye and estimated natural fluorescence lifetimes $\tau$ in nanoseconds of the first excited electronic levels according to formula from W. Zou, WJ Liu, J. Comput. Chem, 26, 106 (2004) for molecules from MS. For natural fluorescence lifetime calculations the averaged TDMs for ground state and excited state equilibrium structures are taken.

| CaOH | | CaNC | |
|---|---|---|---|
| Equilibrium structure | TDM | Equilibrium structure | TDM |
| X ($^2\Sigma$) | 6.47 | X ($^2\Sigma$) | 6.04 |
| A ($^2\Pi$) | 6.51 | A ($^2\Pi$) | 6.07 |
| $\tau$ = 22 | | $\tau$ = 21 | |

| $MgCH_3$ | | $CaCH_3$ | |
|---|---|---|---|
| Equilibrium structure | TDM | Equilibrium structure | TDM |
| X ($^2A_1$) | 3.43 | X ($^2A_1$) | 5.83 |
| A ($^2E$) | 3.26 | A ($^2E$) | 5.83 |
| $\tau$ = 31 | | $\tau$ = 34 | |

TABLE IV. Harmonic vibrational wavenumbers $\tilde{\omega}_e$ for normal modes $\nu_l$ of MgCHDT in inverse centimetres.

MgCHDT

| State | Normal modes $\nu_l$ | | State | Normal modes $\nu_l$ | |
|---|---|---|---|---|---|
| X ($^2A_1$) | $\nu_1(a_1)$ | 3157 | A ($^2E$) | $\nu_1(a_1)$ | 3185 |
| | $\nu_2(a_1)$ | 2297 | | $\nu_2(a_1)$ | 2338 |
| | $\nu_3(a_1)$ | 1936 | | $\nu_3(a_1)$ | 1956 |
| | $\nu_4(a_1)$ | 1356 | | $\nu_4(a_1)$ | 1197 |
| | $\nu_5(a_1)$ | 1178 | | $\nu_5(a_1)$ | 1064 |
| | $\nu_6(a_1)$ | 941 | | $\nu_6(a_1)$ | 852 |
| | $\nu_7(a_1)$ | 567 | | $\nu_7(a_1)$ | 524 |
| | $\nu_8(a_1)$ | 516 | | $\nu_8(a_1)$ | 432 |
| | $\nu_9(a_1)$ | 443 | | $\nu_9(a_1)$ | 297 |

### A. Electronic structure calculations

The details of electronic structure calculations with MOLPRO program package are provided below. The meaning of the input parameters is following (on the example of CaOH):

```
MCSCF(occ,20; frozen,11;wf,29,1,1;state,5) /def2-QZVPP
```

all calculations are performed with the basis set of def2-QZVPP quality taken from MOLPRO basis set library `http://www.molpro.net/info/basis.php?portal=user&choice=Basis+library`. The atomic basis set on Ca includes functions [24s,18p,6d,3f]/[11s,6p,4d,3f], so 24 primitive gaussians of $s$-type, 18 of $p$-type, 6 of $d$-type and 3 of $f$-type are contracted to 11 $s$-functions, 6 $p$-functions, 4 $d$-functions and 3 $f$-functions. Analogously atomic basis sets on O consists of [15s,8p,3d,2f,1g]/[7s,4p,3d,2f,1g] functions and on H [7s,3p,2d,1f]/[4s,3p,2d,1f]. Using these atomic basis sets closed-shell Hartree-Fock calculation of the single charged cation (with 28 electrons filling energetically lowest orbitals) of CaOH is performed to obtain a set of molecular one-electron orbitals. Then 29 electrons are distributed in molecular orbital subspaces as following: 22 electrons are frozen on 11 lowest orbitals, these orbitals are not optimised during calculations. 7 electrons are distributed among next 9 orbitals following by energy after frozen orbitals. In CASSCF calculations both shape of these orbitals is optimised and weights of all possible configurational wave functions which can be generated from the given set of electrons and active orbitals. In the variational procedure the minimum of the sum of the weighted energies of a few lowest-lying doublet states is searched for (5 in the given example). Then optimisation of the structure of either ground (X) or excited (A) state is performed using given electronic structure method and vibrational analyses is made at equilibrium structures. As a result the normal coordinates and harmonic vibrational frequencies can be computed. This information is later used in FC factor calculations by HOTFCHT code. Analogously for internally contracted configuration interaction scheme (see [9]):

```
HF/CI(occ,16; core,6; wf,29,1,1; state,2),
```

after Hartree-Fock (HF) calculations of the molecular cation, the internally contracted CI method is used to obtain the energies and molecular properties. The internal configuration space consists of 16 orbitals, but 6 of them are frozen, so they are always doubly occupied and no excitations are allowed from them. Other 10 orbitals span the internal configuration space with 17 electrons (29-6*2=17) allowing to occupy any of them. Then external configuration state functions (CSF) are generated by applying single and double excitation operators to internal CI states (2 in this case) and then eigenfunctions of the molecular hamiltonian are found on the basis of all available CSF's. Typical the number of CSF's varies from a few hundred thousands to a few millions. Analogous notation and procedure are used in calculations of CaNC, $CaCH_3$, $MgCH_3$ and MgCHDT.

---

[1] M. Li and J. Coxon, J. Chem. Phys. **104**, 4961 (1996).
[2] C. Scurlock, D. Fletcher, and T. Steimle, J. Chem. Phys. **101**, 7255 (1994), ISSN 0021-9606.
[3] C. Bauschlicher, S. Langhoff, T. Steimle, and J. Shirley, J. Chem. Phys. **93**, 4179 (1990), ISSN 0021-9606.
[4] T. Steimle, D. Fletcher, K. Jung, and C. Scurlock, J. Chem. Phys. **96**, 2556 (1992).
[5] P. F. Bernath and C. R. Brazier, Astrophysical Journal **288**, 373 (1985).
[6] R. Rubino, J. Williamson, and T. Miller, J. Chem. Phys. **103**, 5964 (1995), ISSN 0021-9606.
[7] C. Brazier and P. Bernath, J. Chem. Phys. **91**, 4548 (1989), ISSN 0021-9606.
[8] A. Marr, F. Grieman, and T. Steimle, J. Chem. Phys. **105**, 3930 (1996), ISSN 0021-9606.
[9] H. Werner and P. Knowles, J. Chem. Phys. **89**, 5803 (1988).

TABLE V. Calculated and experimental molecular parameters for CaOH. Internuclear distances $R_i$ are given in Å, electric dipole moments in Debye, transition wavenumbers $T_e$ and harmonic vibrational wavenumbers $\tilde{\omega}_e$ for normal modes $\nu_l$ in inverse centimetres.

| Molecule | Method/Basis | State/Structure (internuclear distances are in Å) | | Vibrational wavenumbers (modes) (inverse centimeters) | |
|---|---|---|---|---|---|
| | | X | | | |
| CaOH | MCSCF(occ, 20; frozen, 11; wf, 29, 1, 1; state, 5) /def2-QZVPP | $R_{(Ca-O)}$ | 2.0038 | $\nu_2(\pi)$ | 411/408 |
| | | $R_{(O-H)}$ | 0.9333 | $\nu_1(\sigma^+)$ | 622 |
| | | ∠ Ca-O-H | 179.97 | $\nu_3(\sigma^+)$ | 4276 |
| | | A | | | |
| | | $R_{(Ca-O)}$ | 1.9769 | $\nu_2(\pi)$ | 402/386 |
| | | $R_{(O-H)}$ | 0.9332 | $\nu_1(\sigma^+)$ | 646 |
| | | ∠ Ca-O-H | 179.97 | $\nu_3(\sigma^+)$ | 4279 |
| | Displacement | $\Delta R_{(Ca-O)}$ | 0.0269 | | |
| | | $\Delta R_{(O-H)}$ | 0.0001 | | |
| | | Δ ∠ Ca-O-H | 0 | | |
| | | X | | | |
| | HF/CI(occ,16; core,6; wf,29,1,1; state,2) /def2-TZVP | $R_{(Ca-O)}$ | 2.0026 | $\nu_2(\pi)$ | 429/429 |
| | | $R_{(O-H)}$ | 0.9456 | $\nu_1(\sigma^+)$ | 623 |
| | | ∠ Ca-O-H | 179.97 | $\nu_3(\sigma^+)$ | 4105 |
| | | A | | | |
| | | $R_{(Ca-O)}$ | 1.9721 | $\nu_2(\pi)$ | 402/403 |
| | | $R_{(O-H)}$ | 0.9456 | $\nu_1(\sigma^+)$ | 651 |
| | | ∠ Ca-O-H | 179.97 | $\nu_3(\sigma^+)$ | 4106 |
| | Displacement | | | | |
| | | $\Delta R_{(Ca-O)}$ | 0.0305 | | |
| | | $\Delta R_{(O-H)}$ | 0.0000 | | |
| | | Δ ∠ Ca-O-H | 0 | | |
| | Experiment[a] | | | | |
| | | X | | | |
| | | $R_{(Ca-O)}$ | 1.9746 | | |
| | | $R_{(O-H)}$ | 0.9562 | | |
| | | ∠ Ca-O-H | 180.0 | | |
| | | A | | | |
| | | $R_{(Ca-O)}$ | 1.9532 | | |
| | | $R_{(O-H)}$ | 0.9572 | | |
| | | ∠ Ca-O-H | 180.0 | | |
| | Displacement | | | | |
| | | $\Delta R_{(Ca-O)}$ | 0.0214 | | |
| | | $\Delta R_{(O-H)}$ | 0.0010 | | |

[a] from [1]

TABLE VI. Calculated and experimental molecular parameters for CaNC. Internuclear distances $R_i$ are given in Å, electric dipole moments in Debye, transition wavenumbers $T_e$ and harmonic vibrational wavenumbers $\tilde{\omega}_e$ for normal modes $\nu_l$ in inverse centimetres.

| Molecule | Method/Basis | State/Structure (internuclear distances are in Å) | | Vibrational wavenumbers (modes) (inverse centimeters) | |
|---|---|---|---|---|---|
| CaNC | MCSCF(occ,22; closed,12; frozen,8; wf,33,1,1; state,3) /def2-TZVP | | | | |
| | | X | | | |
| | | $R_{(Ca-N)}$ | 2.2431 | $\nu_2(\pi)$ | 78/78 |
| | | $R_{(N-C)}$ | 1.1864 | $\nu_1(\sigma^+)$ | 409 |
| | | ∠ Ca-N-C | 179.97 | $\nu_3(\sigma^+)$ | 2069 |
| | | A | | | |
| | | $R_{(Ca-N)}$ | 2.2167 | $\nu_2(\pi)$ | 59/76 |
| | | $R_{(N-C)}$ | 1.1831 | $\nu_1(\sigma^+)$ | 424 |
| | | ∠ Ca-N-C | 179.97 | $\nu_3(\sigma^+)$ | 2091 |
| | Displacement | | | | |
| | | Δ $R_{(Ca-N)}$ | 0.0264 | | |
| | | Δ $R_{(N-C)}$ | 0.0033 | | |
| | | Δ ∠ Ca-N-C | 0.0 | | |
| | MCSCF(occ,22; closed,12; frozen,8; wf,33,1,1; state,3) /def2-QZVPP | | | | |
| | | X | | | |
| | | $R_{(Ca-N)}$ | 2.2344 | $\nu_2(\pi)$ | 85/85 |
| | | $R_{(N-C)}$ | 1.1866 | $\nu_1(\sigma^+)$ | 412 |
| | | ∠ Ca-N-C | 179.54 | $\nu_3(\sigma^+)$ | 2062 |
| | | A | | | |
| | | $R_{(Ca-N)}$ | 2.2076 | $\nu_2(\pi)$ | 63/63 |
| | | $R_{(N-C)}$ | 1.1861 | $\nu_1(\sigma^+)$ | 426 |
| | | ∠ Ca-N-C | 179.97 | $\nu_3(\sigma^+)$ | 2066 |
| | Displacement | | | | |
| | | Δ $R_{(Ca-N)}$ | 0.0268 | | |
| | | Δ $R_{(N-C)}$ | 0.0005 | | |
| | | Δ ∠ Ca-N-C | −0.43 | | |
| | Experiment[a] | | | | |
| | | X | | | |
| | | $R_{(Ca-N)}$ | 2.2065 | | |
| | | $R_{(N-C)}$ | 1.1186 | | |
| | | ∠ Ca-N-C | 180.0 | | |

[a] from [2]

TABLE VII. Calculated and experimental molecular parameters for $CaCH_3$. Internuclear distances $R_i$ are given in Å, electric dipole moments in Debye, transition wavenumbers $T_e$ and harmonic vibrational wavenumbers $\tilde{\omega}_e$ for normal modes $\nu_l$ in inverse centimetres. Imaginary wavenumbers imply that on the given normal coordinate the point with minimal energy has not been reached.

| Molecule | Method/Basis | State/Structure (internuclear distances are in Å) | | Vibrational wavenumbers (modes) (inverse centimeters) | |
|---|---|---|---|---|---|
| $CaCH_3$ [a] | MCSCF(occ, 15; frozen, 6; wf, 29, 1, 1; state, 1) / CI (occ, 20; core, 11; wf, 29, 1, 1; state, 3) / def2–TZVP | | | | |
| | | X | | | |
| | | $R_{(Ca-C)}$ | 2.4206 | $\nu_6$ (e) | 367/367 |
| | | $R_{(C-H)}$ | 1.0945 | $\nu_5$ (e) | 1495/1495 |
| | | ∠ Ca-C-H | 113.40 | $\nu_4$ (e) | 3045/3045 |
| | | | | $\nu_3$ ($a_1$) | 418 |
| | | | | $\nu_2$ ($a_1$) | 1187 |
| | | | | $\nu_1$ ($a_1$) | 3035 |
| | | A | | | |
| | | $R_{(Ca-C)}$ | 2.4052 | $\nu_6$ (e) | 534 i/925 i |
| | | $R_{(C-H)}$ | 1.089 | $\nu_5$ (e) | 1300 i/1617 i |
| | | ∠ Ca-C-H | 112.02 | $\nu_4$ (e) | 2436/2776 |
| | | | | $\nu_3$ ($a_1$) | 435 |
| | | | | $\nu_2$ ($a_1$) | 1153 |
| | | | | $\nu_1$ ($a_1$) | 2863 |
| | | $T_e$ | 16081 | | |
| | Experiment[b] | | | | |
| | | X | | | |
| | | $R_{(Ca-C)}$ | 2.349(13) | | |
| | | $R_{(C-H)}$ | 1.100(20) | | |
| | | ∠ Ca-C-H | 113.11 | | |
| | | $\theta$ H-C-H | 120.0 | | |
| | | A | | | |
| | | $R_{(Ca-C)}$ | 2.353(14) | | |
| | | $R_{(C-H)}$ | 1.100(20) | | |
| | | ∠ Ca-C-H1 | 109.74 | | |
| | | $\theta$ H1-C-H2 | 120.0 | | |
| | | $T_e$ | 14743 | | |
| | Displacement | | | | |
| | | $\Delta R_{(Ca-C)}$ | −0.004 | | |
| | | $\Delta$ $R_{(C-H)}$ | −0.01 | | |
| | | $\Delta$ ∠ Ca-C-H | 3.37 | | |

[a] in $C_{3v}$ symmetry
[b] from [7]

TABLE VIII. Calculated molecular parameters for $MgCH_3$. Internuclear distances $R_i$ are given in Å, electric dipole moments in Debye, transition wavenumbers $T_e e$ and harmonic vibrational wavenumbers $\tilde{\omega}_e$ for normal modes $\nu_l$ in inverse centimetres.

| Molecule | Method/Basis | State/Structure (internuclear distances are in Å) | | Vibrational wavenumbers (modes) [a] (inverse centimeters) | |
|---|---|---|---|---|---|
| $MgCH_3$ | MCSCF ( occ, 11; frozen, 2 ; wf, 21, 1, 1; state, 1) / CI ( occ, 14; core, 6; wf, 21, 1, 1; state, 2 ) / def2-TZVP | | | | |
| | | X | | | |
| | | $R_{(Mg-C)}$ | 2.1205 | $\nu_6$ (e) | 639/685 |
| | | $R_{(C-H1)}=R_{(C-H2)}=R_{(C-H3)}$ | 1.0930 | $\nu_5$ (e) | 1535/1564 |
| | | ∠ Mg-C-H1 | 111.24 | $\nu_4$ (e) | 3145/3172 |
| | | ∠ Mg-C-H2=∠ Mg-C-H3 | 111.23 | $\nu_3$ ($a_1$) | 498 |
| | | $\theta$ H1-C-H2 | 120.00 | $\nu_2$ ($a_1$) | 1165 |
| | | $\theta$ H1-C-H3 | 239.99 | $\nu_3$ ($a_1$) | 3083 |
| | | A | | | |
| | | $R_{(Mg-C)}$ | 2.1629 | $\nu_6$ (e) | 426/449 |
| | | $R_{(C-H1)}=R_{(C-H2)}$ | 1.084 | $\nu_5$ (e) | 1386/1478 |
| | | $R_{(C-H3)}$ | 1.087 | $\nu_4$ (e) | 3204/3218 |
| | | ∠ Mg-C-H1 | 107.88 | $\nu_3$ ($a_1$) | 627 |
| | | ∠ Mg-C-H2 | 107.79 | $\nu_2$ ($a_1$) | 1048 |
| | | ∠ Mg-C-H3 | 104.54 | $\nu_1$ ($a_1$) | 3108 |
| | | $\theta$ H1-C-H2 | 118.97 | | |
| | | $\theta$ H1-C-H3 | 237.84 | | |
| | Displacement | | | | |
| | | $\Delta$ $R_{(Mg-C)}$ | −0.0424 | | |
| | | $\Delta$ $R_{(C-H1)}$= $\Delta$ $R_{(C-H2)}$ | 0.09 | | |
| | | $\Delta$ $R_{(C-H3)}$ | 0.006 | | |

[a] approximate vibrational symmetry in parentheses

TABLE IX. Calculated molecular parameters for $MgCH_3$ in $C_{3v}$ symmetry. Internuclear distances $R_i$ are given in Å, electric dipole moments in Debye, transition wavenumbers $T_e$ and harmonic vibrational wavenumbers $\tilde{\omega}_e$ for normal modes $\nu_l$ in inverse centimetres. Imaginary wavenumbers imply that on the given normal coordinate the point with minimal energy has not been reached.

| Molecule | Method/Basis | State/Structure (internuclear distances are in Å) | | Vibrational wavenumbers (modes) [a] (inverse centimeters) | |
|---|---|---|---|---|---|
| $MgCH_3$ | MCSCF ( occ, 11; frozen, 2 ; wf, 21, 1, 1; state, 1) / CI ( occ, 14; core, 6; wf, 21, 1, 1; state, 3 ) / def2-TZVP | | | | |
| | | X | | | |
| | | $R_{(Mg-C)}$ | 2.1204 | $\nu_6$ (e) | 511/511 |
| | | $R_{(C-H1)}=R_{(C-H2)}=R_{(C-H3)}$ | 1.0932 | $\nu_5$ (e) | 1481/1481 |
| | | ∠ Mg-C-H1= ∠ Mg-C-H2=∠ Mg-C-H3 | 111.2 | $\nu_4$ (e) | 3126/3126 |
| | | $\theta$ H-C-H | 120.00 | $\nu_3$ ($a_1$) | 511 |
| | | | | $\nu_2$ ($a_1$) | 1154 |
| | | | | $\nu_1$ ($a_1$) | 3043 |
| | | A | | | |
| | | $R_{(Mg-C)}$ | 2.1637 | $\nu_6$ (e) | 1202i/1692i |
| | | $R_{(C-H1)}=R_{(C-H2)}=R_{(C-H3)}$ | 1.0851 | $\nu_5$ (e) | 1899/2099 i |
| | | ∠ Mg-C-H1= ∠ Mg-C-H2=∠ Mg-C-H3 | 106.73 | $\nu_4$ (e) | 2433/2546 i |
| | | $\theta$ H-C-H | 120.00 | $\nu_3$ ($a_1$) | 443 |
| | | | | $\nu_2$ ($a_1$) | 1089 |
| | | | | $\nu_1$ ($a_1$) | 2605 |
| | Displacement | | | | |
| | | $\Delta R_{(Mg-C)}$ | −0.0433 | | |
| | | $\Delta R_{(C-H1)}= \Delta R_{(C-H2)}=\Delta R_{(C-H3)}$ | 0.0079 | | |

[a] vibrational symmetry in parentheses

TABLE X. Calculated molecular parameters for $MgCH_3$. Internuclear distances $R_i$ are given in Å, electric dipole moments in Debye, transition wavenumbers $T_e$ and harmonic vibrational wavenumbers $\tilde{\omega}_e$ for normal modes $\nu_l$ in inverse centimetres.

| Molecule | Method/Basis | State/Structure (internuclear distances are in Å) | | Vibrational wavenumbers (modes) [a] (inverse centimeters) | |
|---|---|---|---|---|---|
| $MgCH_3$ | MCSCF ( occ, 15; frozen, 6; wf, 21, 1, 1; state, 3) / def2-QZVPP | | | | |
| | | X | | | |
| | | $R_{(Mg-C)}$ | 2.1590 | $\nu_6$ (e) | 519/520 |
| | | $R_{(C-H1)}=R_{(C-H2)}$ | 1.0843 | $\nu_5$ (e) | 1514/1544 |
| | | $R_{(C-H3)}$ | 1.1085 | $\nu_4$ (e) | 2926/3206 |
| | | ∠ Mg-C-H1 | 109.26 | $\nu_3$ ($a_1$) | 462 |
| | | ∠ Mg-C-H2=∠ Mg-C-H3 | 110.98 | $\nu_2$ ($a_1$) | 1175 |
| | | $\theta$ H1-C-H2 | 121.46 | $\nu_1$ ($a_1$) | 3159 |
| | | $\theta$ H1-C-H3 | 240.73 | | |
| | | A | | | |
| | | $R_{(Mg-C)}$ | 2.2590 | $\nu_6$ (e) | 451/596 |
| | | $R_{(C-H1)}=R_{(C-H2)}$ | 1.0737 | $\nu_5$ (e) | 1412/1538 |
| | | $R_{(C-H3)}$ | 1.1002 | $\nu_4$ (e) | 3273/3306 |
| | | | | $\nu_3$ ($a_1$) | 350 |
| | | | | $\nu_2$ ($a_1$) | 1047 |
| | | | | $\nu_1$ ($a_1$) | 3017 |
| | Displacement | | | | |
| | | $\Delta$ $R_{(Mg-C)}$ | −0.100 | | |
| | | $\Delta$ $R_{(C-H1)}$= $\Delta$ $R_{(C-H2)}$ | 0.0106 | | |
| | | $\Delta$ $R_{(C-H3)}$ | 0.0083 | | |

[a] approximate vibrational symmetry in parentheses

TABLE XI. Experimental molecular parameters for $MgCH_3$. Internuclear distances $R_i$ are given in Å, electric dipole moments in Debye, transition wavenumbers $T_e$ and harmonic vibrational wavenumbers $\tilde{\omega}_e$ for normal modes $\nu_l$ in inverse centimetres.

| Molecule | Method/Basis | State/Structure (internuclear distances are in Å) | | Vibrational wavenumbers (modes) (inverse centimeters) |
|---|---|---|---|---|
| $MgCH_3$ | Experiment[a] | | | |
| | | X | | |
| | | $R_{(Mg-C)}$ | 2.102 | |
| | | $R_{(C-H)}$ | 1.105 [b] | |
| | | A | | |
| | | $R_{(Mg-C)}$ | 2.124 | |
| | | $R_{(C-H)}$ | 1.105 [b] | |
| | Displacement | | | |
| | | $\Delta$ $R_{(Mg-C)}$ | −0.022 | |
| | | $\Delta$ $R_{(C-H)}$ | 0 | |

[a] from [6]
[b] in [6] this value is fixed from theoretical calculations by G.Gawboy
